# Supplementary material for: Minimizing the average distance to a closest leaf in a phylogenetic tree
Source: arXiv:1205.6867 source file (2012-08-31)
Supplement: Supplementary file 1 [file voro_suppfig.pdf]

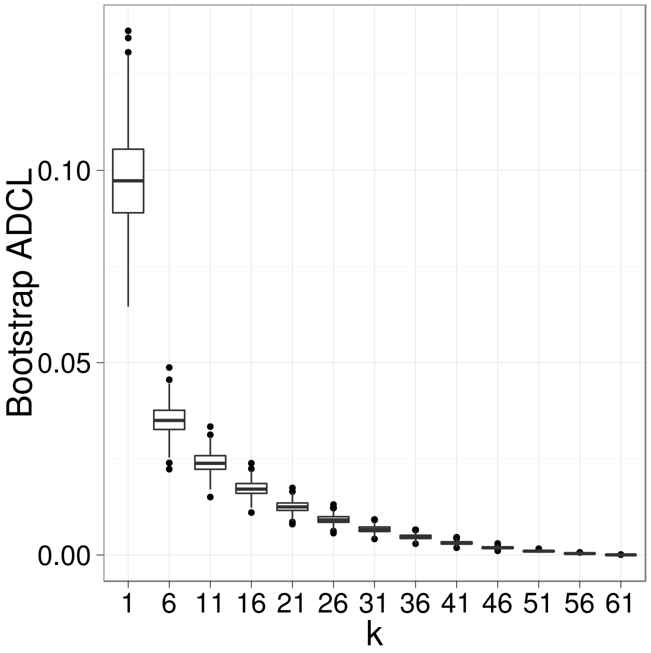


FIGURE S1. The distribution of ADCL values under 500 bootstrap replicates for the 65 non-chimeric Enterobacteriaceae sequences used elsewhere in the paper.

FIGbootstrap

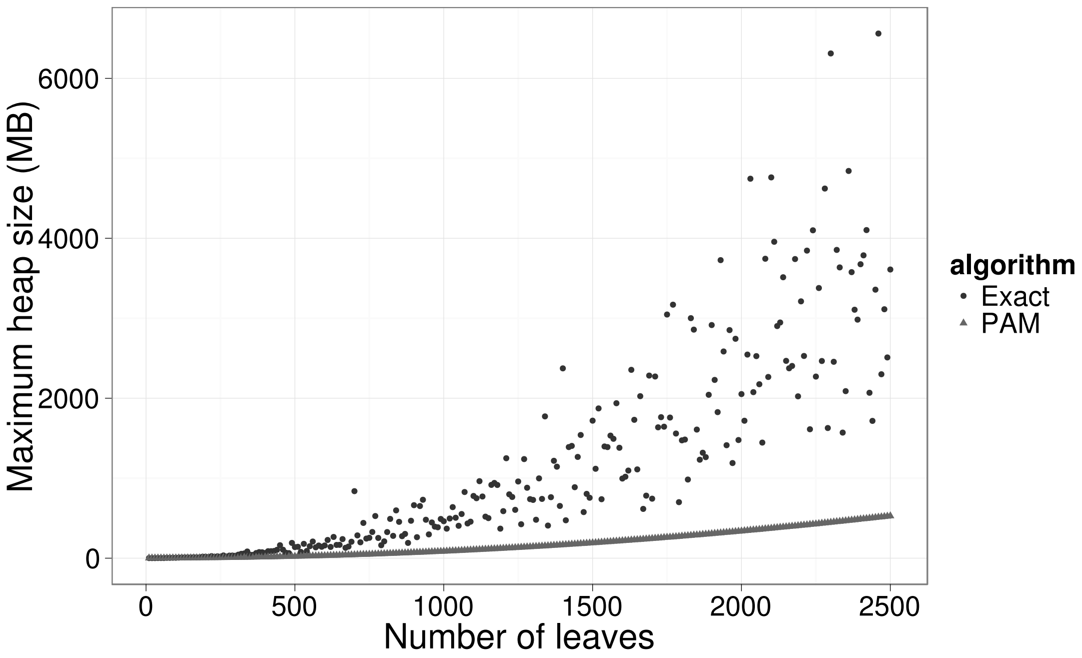


FIGURE S2. Comparison of the memory required to run the exact algorithm versus PAM with respect to the number of leaves in the original tree. Trees were generated as in Figure 7. The peak heap memory usage for each algorithm on a given tree is shown by a single point.

FIGnMemoryComplexity

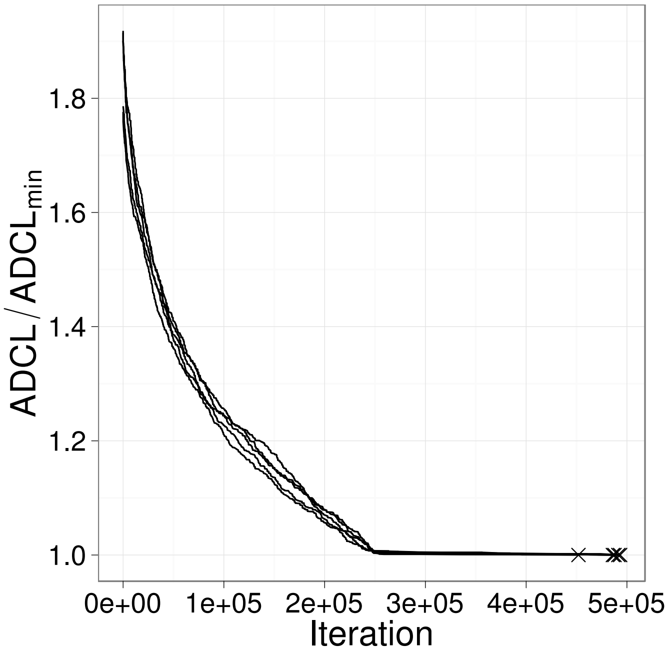


Figure S3. PAM convergence on the five 1000-leaf trees described in Figure 6. Each iteration is an attempt to swap a medoid from the current partition with a non-medoid. Crosses denote the iteration at which the algorithm converged.

FIGpamCostPerIter

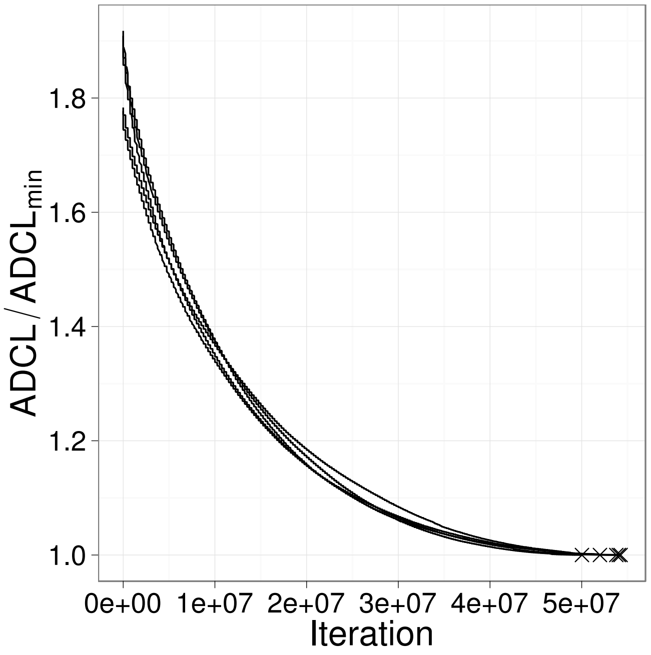


Figure S4. Convergence of the traditional PAM algorithm on the five 1000-leaf trees described in Figure 6. Each iteration is an attempt to swap a medoid from the current partition with a non-medoid. Crosses denote the iteration at which the algorithm converged.

FIGtradPamCostPerIter
