# Supplementary material for: Minimizing the average distance to a closest leaf in a phylogenetic tree
Source: arXiv:1205.6867 source file (2012-08-31)
Supplement: Supplementary file 2 [file xvoro_suppfig.tex]

\documentclass{amsart}

\usepackage{amsmath,amsfonts,amssymb,amsthm}
\usepackage[english]{babel}
\usepackage{graphicx}
\usepackage{url}
\usepackage[round]{natbib}

% show keys for eqs, etc.
\usepackage[notref,notcite]{showkeys}

% Labels for supplementary materials

% References from main text

\newcommand{\refFIGkTimeComplexity}{6}
\newcommand{\refFIGnTimeComplexity}{7}

% Supplementary figures
\newcommand{\FIGbootstrap}{\
\begin{figure}[ht]
\begin{center}
  \includegraphics[height=9cm]{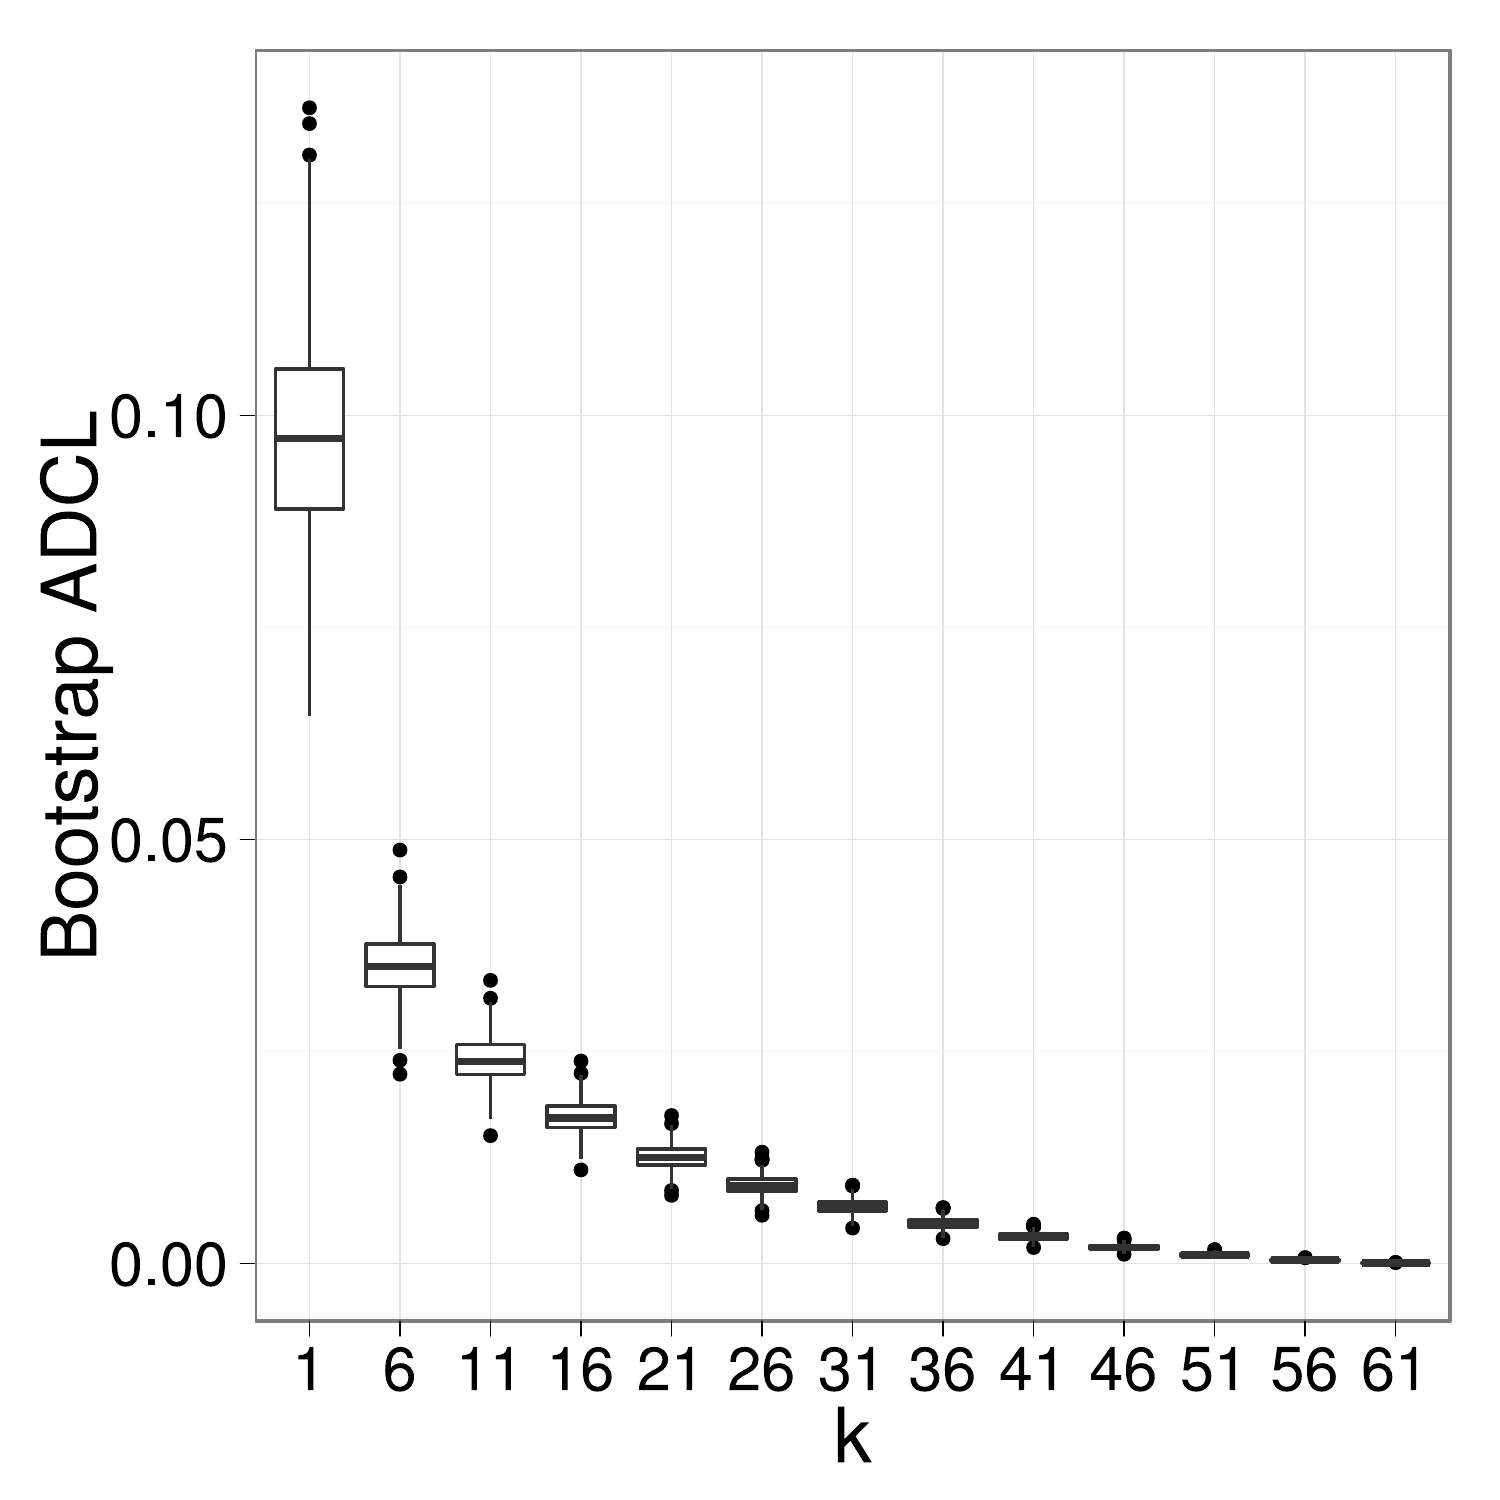}
\end{center}
\caption{\
  The distribution of ADCL values under 500 bootstrap replicates for the 65 non-chimeric Enterobacteriaceae sequences used elsewhere in the paper.
}
\label{FIGbootstrap}
\end{figure}
}

\newcommand{\FIGnMemoryComplexity}{\
\begin{figure}[ht]
\begin{center}
  \includegraphics[height=9cm]{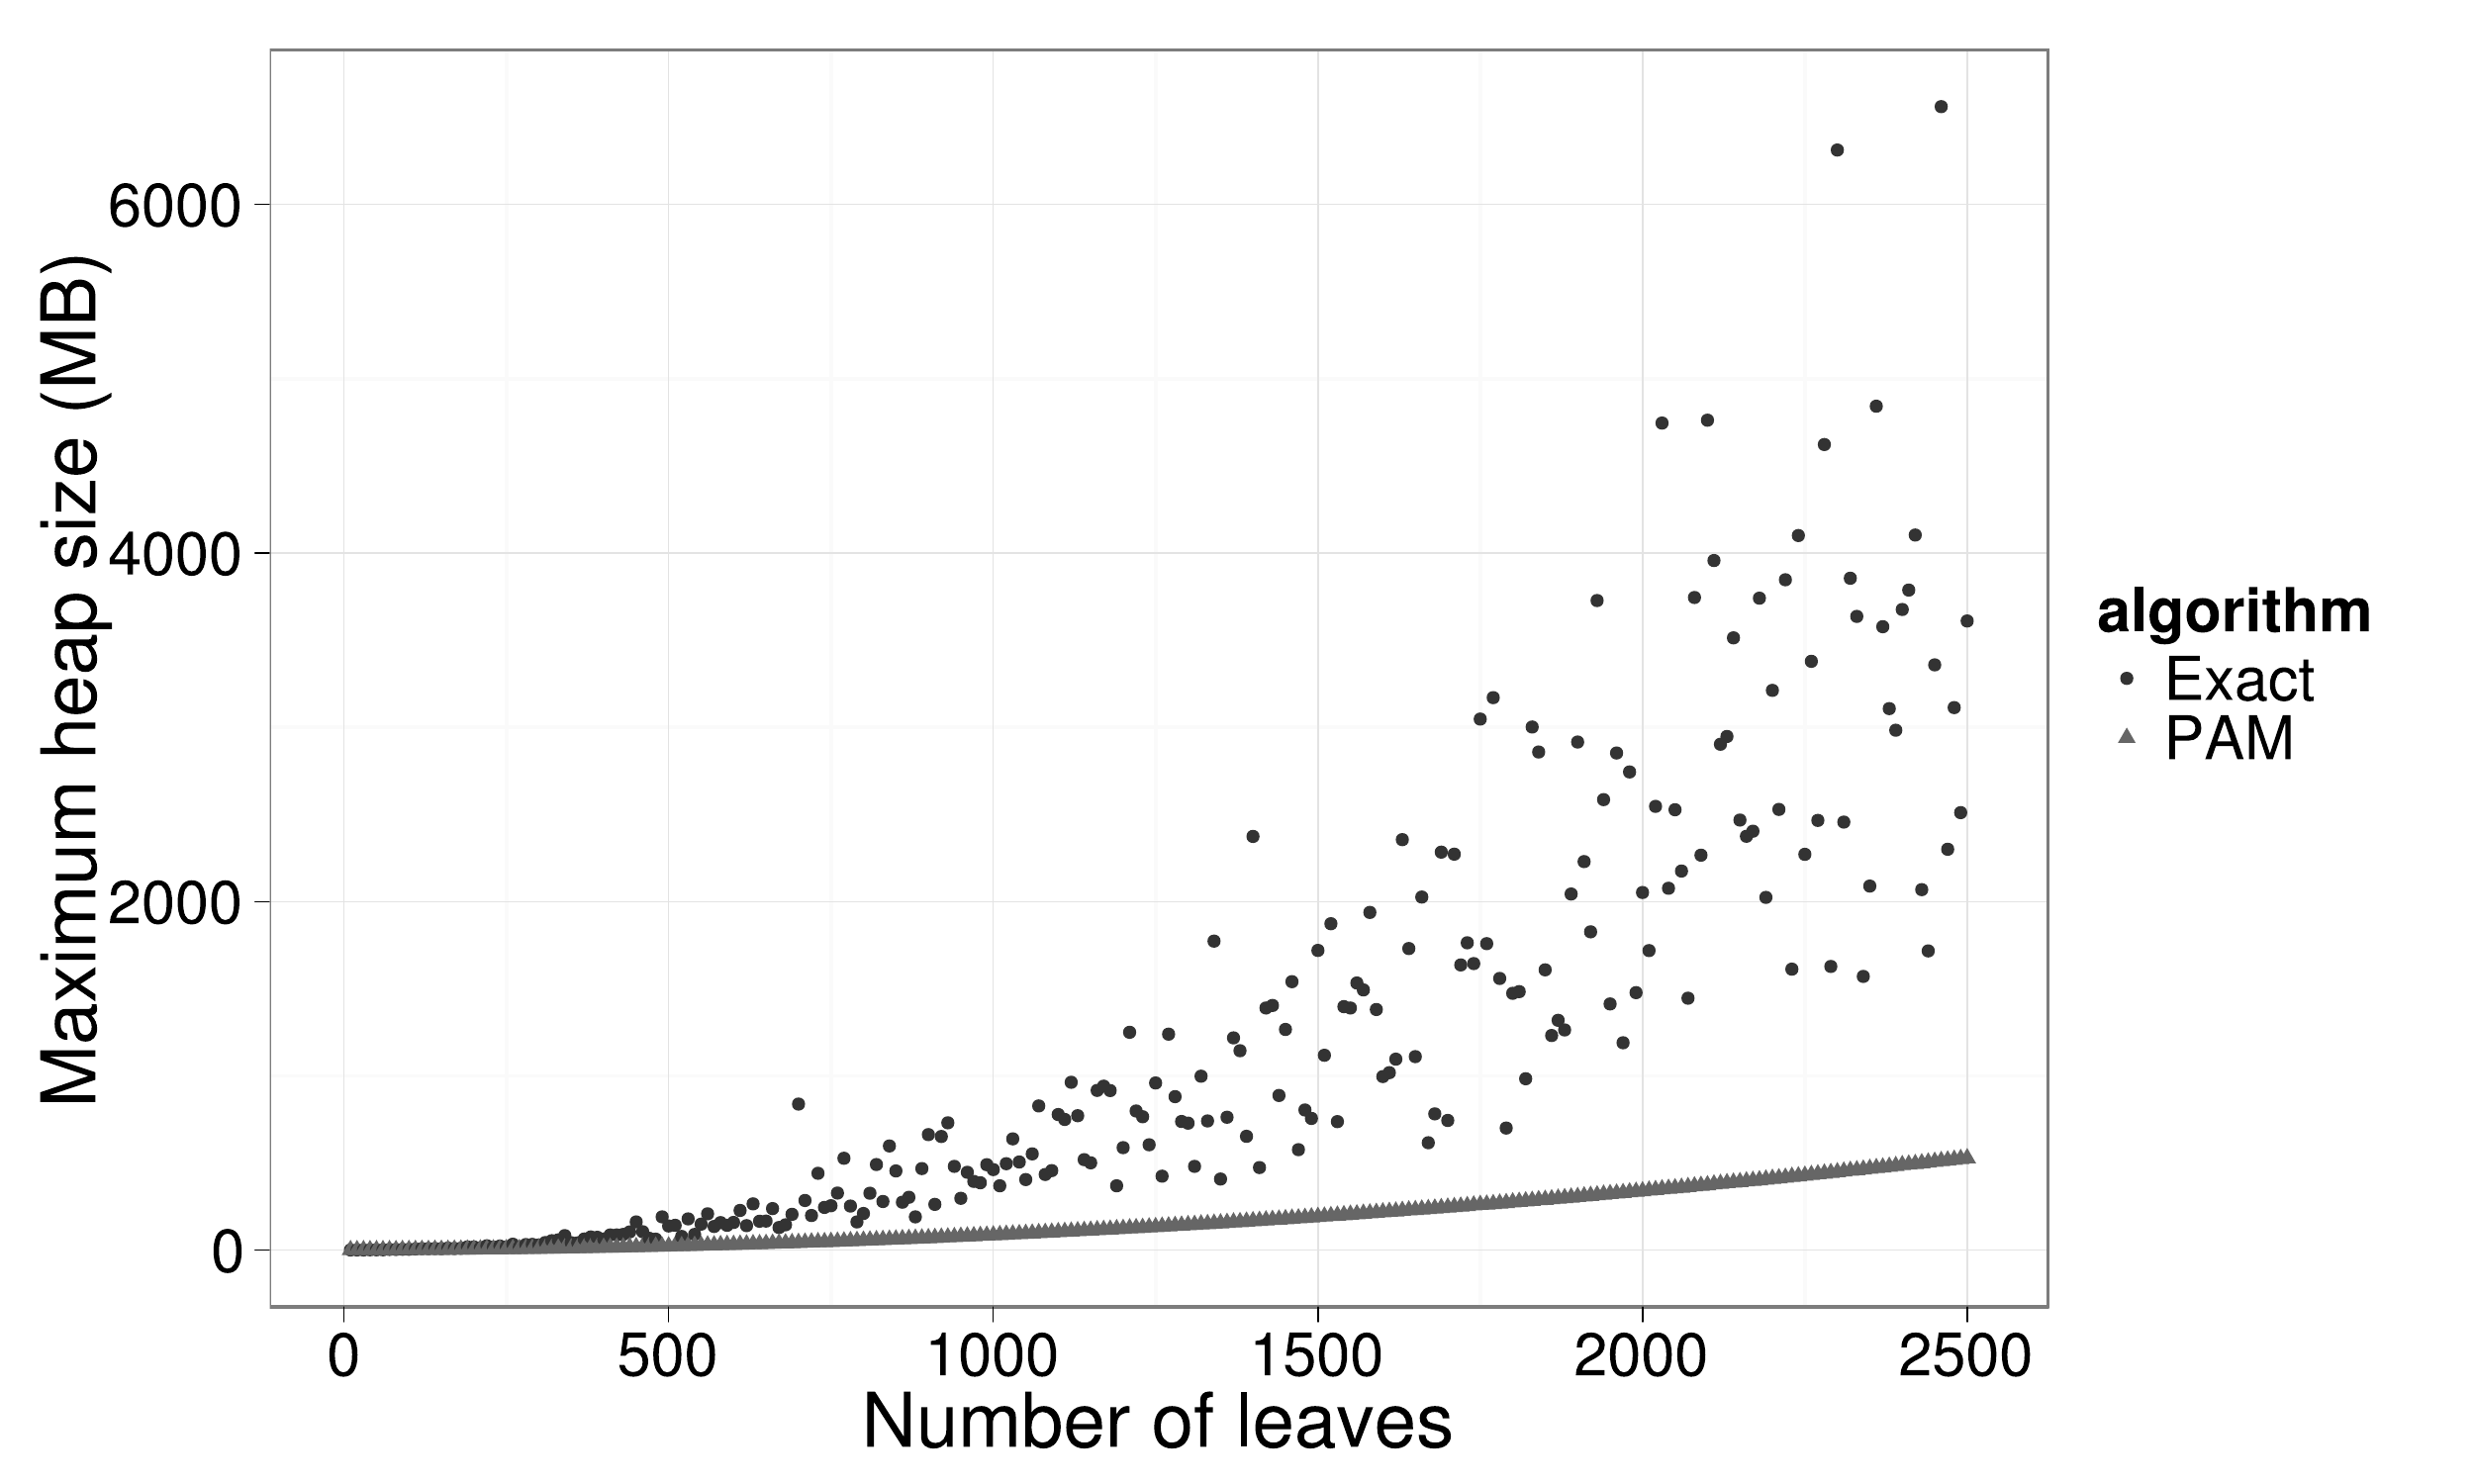}
\end{center}
\caption{\
  Comparison of the memory required to run the exact algorithm versus PAM with respect to the number of leaves in the original tree.
  Trees were generated as in Figure~\refFIGnTimeComplexity.
  The peak heap memory usage for each algorithm on a given tree is shown by a single point.
}
\label{FIGnMemoryComplexity}
\end{figure}
}

\newcommand{\FIGpamCostPerIter}{\
\begin{figure}[ht]
\begin{center}
  \includegraphics[height=9cm]{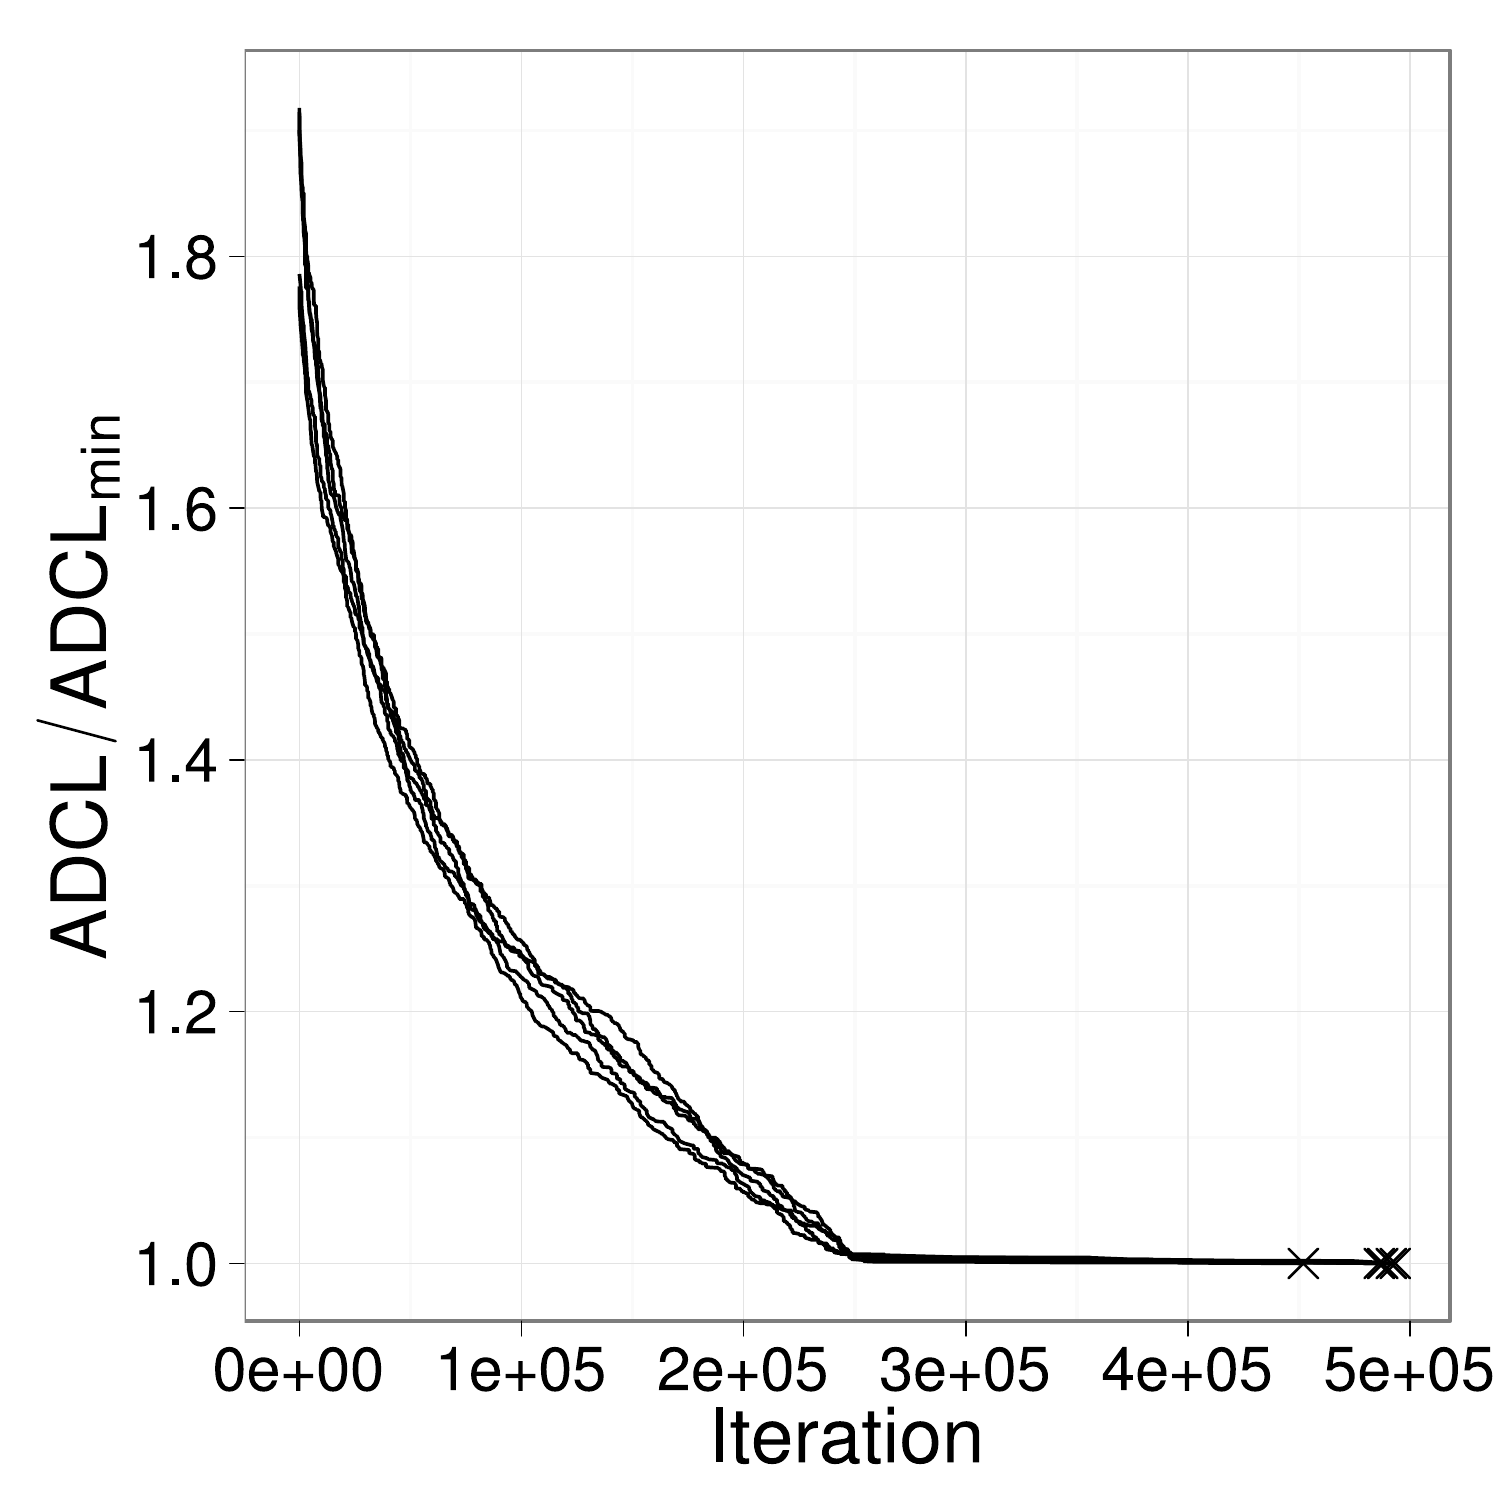}
\end{center}
\caption{\
    PAM convergence on the five 1000-leaf trees described in Figure~\refFIGkTimeComplexity.
    Each iteration is an attempt to swap a medoid from the current partition with a non-medoid.
    Crosses denote the iteration at which the algorithm converged.
}
\label{FIGpamCostPerIter}
\end{figure}
}

\newcommand{\FIGtradPamCostPerIter}{\
\begin{figure}[ht]
\begin{center}
  \includegraphics[height=9cm]{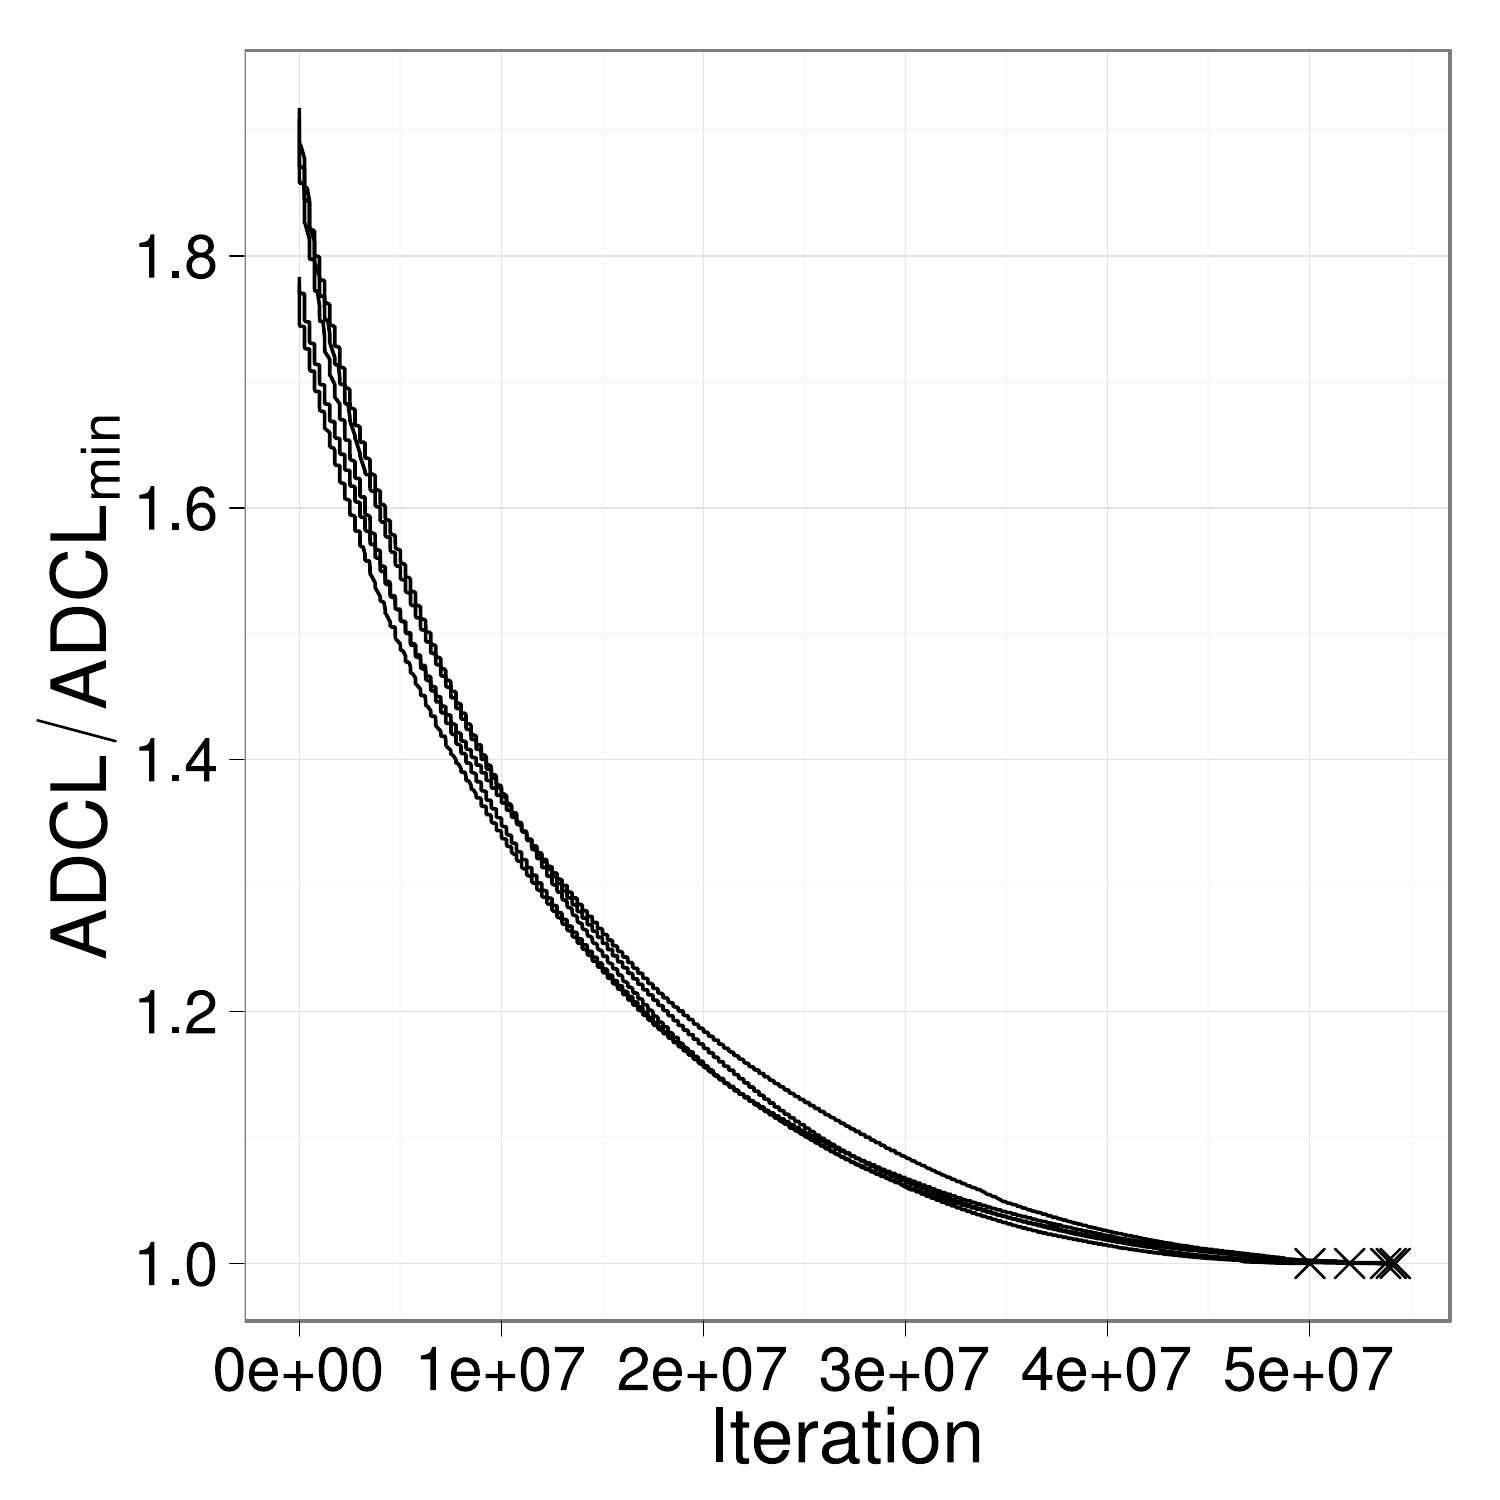}
\end{center}
\caption{\
    Convergence of the traditional PAM algorithm on the five 1000-leaf trees described in Figure~\refFIGkTimeComplexity.
    Each iteration is an attempt to swap a medoid from the current partition with a non-medoid.
    Crosses denote the iteration at which the algorithm converged.
}
\label{FIGtradPamCostPerIter}
\end{figure}
}

\begin{document}

\FIGbootstrap

\newpage

\FIGnMemoryComplexity

\newpage

\FIGpamCostPerIter

\newpage

\FIGtradPamCostPerIter

\end{document}
